# Supplementary material for: A three-dimensional model of skeletal muscle tissues
Source: arXiv:2207.02421 source file (2022-07-06)
Supplement: Supplementary file 1 [file appendix.tex]

% \section{Parameter values for example in \autoref{section:3dmusclecv}}\label{appendix:isometric}
% % \input{Manuscript/isometric.tex}

% \section{Parameter values for example in \autoref{section:3dmuscledynamicexp}}\label{appendix:dynamic}
% % \input{Manuscript/dynamic}
